# Supplementary material for: Complex electric double layers in charged topological colloids
Source: arXiv:1809.04688 ancillary file (2018-09-12)
Supplement: Supplementary file 1 [file Supplementary.pdf]

# Supplementary material: Complex electric double layers in charged topological colloids

J. C. Everts[1,*] and M. Ravnik[1,2]

[1] *Department of Physics, Faculty of Mathematics and Physics, University of Ljubljana, Jadranska 19, 1000 Ljubljana, Slovenia*

[2] *Department of Condensed Matter Physics, Jozef Stefan Institute, Jamova 39, 1000 Ljubljana, Slovenia*

(Dated: September 12, 2018)

* jeffrey.everts@gmail.com

**Constant-charge boundary conditions** In this paper we focussed on constant-potential boundary conditions, see Eq. (2) main text, which resulted in an inhomogeneous surface charge distribution on the particle. If we would instead fix the surface charge density $\sigma$ to be spatially constant, however, the surface potential is inhomogeneous. In this case the constant-charge boundary condition reads

$$\mathbf{n} \cdot \left(\frac{\epsilon_p}{\epsilon_s}\right) \nabla\phi(\mathbf{r})|_{\text{in}} - \mathbf{n} \cdot \nabla\phi(\mathbf{r})|_{\text{out}} = 4\pi\lambda_B\sigma, \quad \mathbf{r} \in \Gamma,$$

with $\epsilon_p$ the dielectric constant of the particle and $\epsilon_s$ the dielectric constant of the surrounding solvent. The exact ratio $\epsilon_p/\epsilon_s$ only affects the surface potential by a few percent, so we fixed it at $\epsilon_p = 2.6$ (PMMA) and $\epsilon_s = 80$ (water), although the exact values are irrelevant within the numerical accuracy that we are interested in. Note, moreover, that for constant-potential boundary conditions the inner gradient vanishes, $\nabla\phi|_{\text{in}} = 0$.

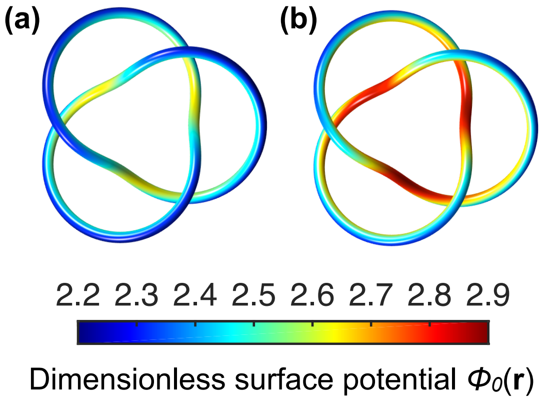


**Figure S1: Surface potential distribution $\Phi_0(\mathbf{r})$ for constant-charge boundary conditions.** We use the same parameters as in Figure 3 for a trefoil knot particle, however with a fixed surface charge density $\sigma$ that coincides with the maximal surface charge density $\sigma_{\max}$ from Figure 3(a) and (b), respectively. Specifically, in (a) we have $\sigma a \lambda_B = 0.083$ and Debye length $\lambda_D = 7.4a$, with $a$ the tube radius and $\lambda_B$ the Bjerrum length. In (b) we have $\sigma a \lambda_B = 0.068$ and $\lambda_D = 11.6a$.

We demonstrate the constant-charge boundary conditions for a trefoil knot particle where we choose $\sigma$ such that it coincides with the maximal charge density $\sigma_{\max}$ of the constant-potential particle in Figure 3. In Figure S1 we see that the resulting surface potential distribution $\Phi_0(\mathbf{r})$ is lowest at the outer rim of the particle tube and close to particle-tube crossings. This is in line with results for spherical particles where it is known that constant-charge particles at low volume fraction have a lower surface potential than at high volume

fractions [1].

Finally, we observed that the topological transformation is exactly the same as in Figure 3 (not shown since isosurfaces are topologically equivalent as in Figure 3(e)), albeit the transition between different topological shapes occur at slightly different Debye lengths. The only difference with the constant-potential result is therefore that isosurfaces of the screening cloud close to the particle surface might not enclose the whole particle, which is an immediate result of the inhomogenous surface-potential distribution $\Phi_0(\mathbf{r})$.

**Screening cloud isosurfaces** In Supplementary movie 1 we show the isosurfaces of Figure 3(e) in the main text from various camera angles.

**Surface charge density of torus knots** In Figure S2 we show the charging behaviour of the torus knots discussed in the main text in Figure 4.

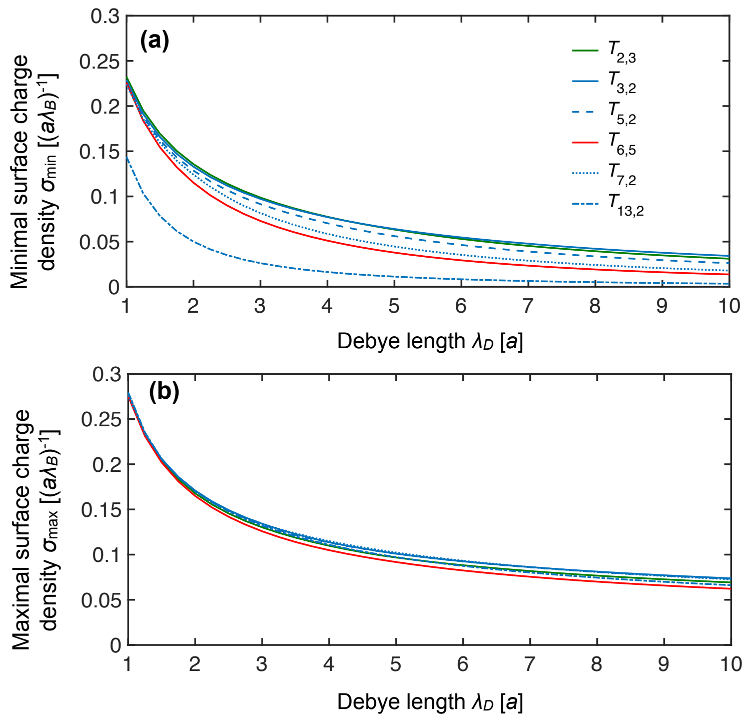


**Figure S2:** (a) Minimal and (b) maximal values of the surface charge density $\sigma_{\min}$ and $\sigma_{\max}$, respectively for various torus knots $T_{p,q}$ for a range of Debye lengths $\lambda_D$ with the same parameters as in Fig. 4. Here $a$ is the tube radius of the torus knot, and $\lambda_B$ is the Bjerrum length of the medium.

[1] Everts, J. C., Boon, N. & van Roij, R. Density-induced reentrant melting of colloidal wigner crystals. *Phys. Chem. Chem. Phys.* **18**, 5211–5218 (2016).
